# Supplementary material for: Drift and Meander of Spiral Waves
Source: arXiv:0912.4247 source file (2009-12-21)
Supplement: Supplementary file 1 [file defs.tex]

\newtheorem{thm}{Theorem}[section]

\theoremstyle{definition}	

\newtheorem{defn}[thm]{Definition}

\newcommand{\ez}{EZ-Freeze }

%%%%%%%%%%%%%%%%% Group Actions etc %%%%%%%%%%%%%%%%%%%%%%%%%%%%%%%%%%%%%%%%

\newcommand{\dd}{\textrm{d}}
\newcommand{\dT}{\textrm{T}(g)}
\newcommand{\ddT}{\textrm{T}(dg)}
\newcommand{\dTddT}{\textrm{T}(g+dg)}
\newcommand{\dTi}{\textrm{T}(g^{-1})}
\newcommand{\ddTi}{\textrm{T}(dg^{-1})}
\newcommand{\ddTcom}{\textrm{T}(\{\textbf{c}dt,\omega dt\})}

%%%%%%%%%%%%%%%%% Bold letters and Symbols %%%%%%%%%%%%%%%%%%%%%%%%%%%%%%%%%%

%Greek

\newcommand{\balp}{\boldsymbol{\alpha}}
\newcommand{\bbet}{\boldsymbol{\beta}}
\newcommand{\bet}{\boldsymbol{\eta}}
\newcommand{\bphi}{\boldsymbol{\phi}}
\newcommand{\bPhi}{\boldsymbol{\Phi}}
\newcommand{\bpsi}{\boldsymbol{\psi}}
\newcommand{\bPsi}{\boldsymbol{\Psi}}

%Latin

\newcommand{\bA}{\textbf{A}}
\newcommand{\bD}{\textbf{B}}
\newcommand{\bc}{\textbf{c}}
\newcommand{\bC}{\textbf{C}}
\newcommand{\be}{\textbf{e}}
\newcommand{\bof}{\textbf{f}}
\newcommand{\boof}{\textbf{f}}
\newcommand{\booF}{\textbf{F}}
\newcommand{\boF}{\textbf{F}(\textbf{V})}
\newcommand{\boFU}{\textbf{F}(\textbf{U})}
\newcommand{\boFt}{\textbf{F}(\textbf{t})}
\newcommand{\bFg}{\textbf{F}_{\mathcal{G}}(\bV)}
\newcommand{\bFm}{\textbf{F}_{\mathcal{M}}(\bV)}
\newcommand{\bg}{\textbf{g}}
\newcommand{\bG}{\textbf{G}}
\newcommand{\bGt}{\textbf{G}(\textbf{t})}
\newcommand{\bh}{\textbf{h}}
\newcommand{\bH}{\textbf{H}}
\newcommand{\bHg}{\til{\bH}_{\mathcal{G}}(\bV,t)}
\newcommand{\bHm}{\til{\bH}_{\mathcal{M}}(\bV,t)}
\newcommand{\bI}{\textbf{I}}
\newcommand{\bk}{\textbf{k}}
\newcommand{\bM}{\textbf{M}}
\newcommand{\bP}{\textbf{P}}
\newcommand{\bp}{\textbf{p}}
\newcommand{\bq}{\textbf{q}}
\newcommand{\bQ}{\textbf{Q}}
\newcommand{\br}{\textbf{r}}
\newcommand{\bR}{\textbf{R}}
\newcommand{\bS}{\textbf{S}}
\newcommand{\bu}{\textbf{u}}
\newcommand{\bU}{\textbf{U}}
\newcommand{\bv}{\textbf{v}}
\newcommand{\bV}{\textbf{V}}
\newcommand{\bw}{\textbf{w}}
\newcommand{\bW}{\textbf{W}}

%%%%%%%%%%%%%%%%% letters with hats and tildes %%%%%%%%%%%%%%%%%

\newcommand{\til}{\tilde}
\newcommand{\bDh}{\hat{\textbf{D}}}
\newcommand{\Bh}{\hat{\partial}}
\newcommand{\hh}{\hat{\textbf{h}}}
\newcommand{\bHt}{\tilde{\textbf{H}}(\textbf{V},t)}
\newcommand{\tH}{\tilde{\textbf{H}}}
\newcommand{\bht}{\tilde{\textbf{h}}}
\newcommand{\btr}{\tilde{\textbf{r}}}
\newcommand{\tx}{\tilde{x}}
\newcommand{\ty}{\tilde{y}}
\newcommand{\tr}{\tilde{r}}
\newcommand{\tbr}{\tilde{\textbf{r}}}
\newcommand{\ttim}{\tilde{t}}
\newcommand{\trho}{\tilde{\rho}}
\newcommand{\tth}{\tilde{\theta}}

%%%%%%%%%%%%%%%%% Derivatives %%%%%%%%%%%%%%%%%%%%%%%%%%%%%%%%%%

\newcommand{\pderiv}[2]{\frac{\partial #1}{\partial #2}} 
\newcommand{\deriv}[2]{\frac{\dd #1}{\dd #2}}

%ODE's

\newcommand{\odcxot}{\frac{\dd{\bc_{x0}}}{\dd{t}}}
\newcommand{\odcyot}{\frac{\dd{\bc_{y0}}}{\dd{t}}}
\newcommand{\odcot}{\frac{\dd{\bc_0}}{\dd{t}}}
\newcommand{\odomt}{\frac{\dd{\omega}}{\dd{t}}}
\newcommand{\odRt}{\frac{\dd{R}}{\dd{t}}}
\newcommand{\odbRt}{\frac{\dd{\bR}}{\dd{t}}}
\newcommand{\odTt}{\frac{\dd{\dT}}{\dd{t}}}
\newcommand{\odTht}{\frac{\dd{\Theta}}{\dd{t}}}
\newcommand{\odThot}{\frac{\dd{\Theta_0}}{\dd{t}}}
\newcommand{\odThonet}{\frac{\dd{\Theta_1}}{\dd{t}}}
\newcommand{\odbut}{\frac{\dd{\bu}}{\dd{t}}}
\newcommand{\odbUt}{\frac{\dd{\bU}}{\dd{t}}}
\newcommand{\odut}{\frac{\dd{\bU}}{\dd{t}}}
\newcommand{\odbvt}{\frac{\dd{\bv}}{\dd{t}}}
\newcommand{\odbVt}{\frac{\dd{\bV}}{\dd{t}}}
\newcommand{\odbVot}{\frac{\dd{\bV_0}}{\dd{t}}}
\newcommand{\odbVpt}{\frac{\dd{\bV_1}}{\dd{t}}}
\newcommand{\odvt}{\frac{\dd{\bV}}{\dd{t}}}
\newcommand{\odbvpit}{\frac{\dd{\bv}_{pi}}{\dd{t}}}
\newcommand{\odbVpit}{\frac{\dd{\bV}_{1pi}}{\dd{t}}}
\newcommand{\odbwt}{\frac{\dd{\bw}}{\dd{t}}}
\newcommand{\odbWt}{\frac{\dd{\bW}}{\dd{t}}}
\newcommand{\odXt}{\frac{\dd{X}}{\dd{t}}}
\newcommand{\odYt}{\frac{\dd{Y}}{\dd{t}}}

%PDE's - wrt x

\newcommand{\pdbvx}{\frac{\partial{\textbf{v}}}{\partial{x}}}
\newcommand{\pdbux}{\frac{\partial{\textbf{u}}}{\partial{x}}}
\newcommand{\pdux}{\frac{\partial{u}}{\partial{x}}}
\newcommand{\pdvx}{\frac{\partial{v}}{\partial{x}}}
\newcommand{\pdvxk}{\frac{\partial{v^{(i)}_k}}{\partial{x}}}
\newcommand{\pduox}{\frac{\partial{\textbf{u}_0}}{\partial{x}}}
\newcommand{\pdvox}{\frac{\partial{\textbf{v}_0}}{\partial{x}}}
\newcommand{\pdbvox}{\frac{\partial{\textbf{v}_0}}{\partial{x}}}
\newcommand{\pdbtvox}{\frac{\partial{\til{\textbf{v}}_0}}{\partial{x}}}
\newcommand{\pdvotx}{\frac{\partial{\textbf{v}_0}}{\partial{\tilde{x}}}}
\newcommand{\pdbvotx}{\frac{\partial{\textbf{v}_0}}{\partial{\til{x}}}}
\newcommand{\pdvoxx}{\frac{\partial^2{\textbf{v}_0}}{\partial{x}^2}}
\newcommand{\pdtrtx}{\frac{\partial{\tilde{\rho}}}{\partial{\tilde{x}}}}
\newcommand{\pdtthtx}{\frac{\partial{\tilde{\theta}}}{\partial{\tilde{x}}}}
\newcommand{\pdtxx}{\frac{\partial{\tilde{x}}}{\partial{x}}}
\newcommand{\pdtyx}{\frac{\partial{\tilde{y}}}{\partial{x}}}
\newcommand{\pdax}{\frac{\partial{\alpha}}{\partial{x}}}

%PDE's - wrt y

\newcommand{\pdbvy}{\frac{\partial{\textbf{v}}}{\partial{y}}}
\newcommand{\pduoy}{\frac{\partial{\textbf{u}_0}}{\partial{y}}}
\newcommand{\pdvoy}{\frac{\partial{\textbf{v}_0}}{\partial{y}}}
\newcommand{\pdbvoy}{\frac{\partial{\textbf{v}_0}}{\partial{y}}}
\newcommand{\pdbvoty}{\frac{\partial{\textbf{v}_0}}{\partial{\til{y}}}}
\newcommand{\pdvoty}{\frac{\partial{\textbf{v}_0}}{\partial{\tilde{y}}}}
\newcommand{\pdvoyy}{\frac{\partial^2{\textbf{v}_0}}{\partial{y}^2}}
\newcommand{\pdtrty}{\frac{\partial{\tilde{\rho}}}{\partial{\tilde{y}}}}
\newcommand{\pdtthty}{\frac{\partial{\tilde{\theta}}}{\partial{\tilde{y}}}}
\newcommand{\pdtxy}{\frac{\partial{\tilde{x}}}{\partial{y}}}
\newcommand{\pdtyy}{\frac{\partial{\tilde{y}}}{\partial{y}}}

%PDE's - wrt theta

\newcommand{\pdbvth}{\frac{\partial{\textbf{v}}}{\partial{\theta}}}
\newcommand{\pdvoth}{\frac{\partial{\textbf{v}_0}}{\partial{\theta}}}
\newcommand{\pdvth}{\frac{\partial{\textbf{v}_1}}{\partial{\theta}}}
\newcommand{\pdvotth}{\frac{\partial{\textbf{v}_0}}{\partial{\tilde{\theta}}}}
\newcommand{\pdvothth}{\frac{\partial^2{\textbf{v}_0}}{\partial{\theta}^2}}

%PDE's - wrt t

\newcommand{\pdvvtt}{\frac{\partial{\textbf{v}}_1}{\partial{\tilde{t}}}}
\newcommand{\pduot}{\frac{\partial{\textbf{u}_0}}{\partial{t}}}
\newcommand{\pdbut}{\frac{\partial{\textbf{u}}}{\partial{t}}}
\newcommand{\pdvot}{\frac{\partial{\textbf{v}_0}}{\partial{t}}}
\newcommand{\pdvott}{\frac{\partial{\textbf{v}_0}}{\partial{\tilde{t}}}}
\newcommand{\pdtthtt}{\frac{\partial{\tilde{\theta}}}{\partial{\tilde{t}}}}
\newcommand{\pdut}{\frac{\partial{\textbf{u}}}{\partial{t}}}
\newcommand{\pdvt}{\frac{\partial{\textbf{v}}}{\partial{t}}}

%PDE's - wrt u/v/U/V

\newcommand{\pdfa}{\frac{\partial{\textbf{f}}}{\partial{\alpha}}}
\newcommand{\pdfu}{\frac{\partial{\textbf{f}}}{\partial{\bu}}}
\newcommand{\pdfvov}{\frac{\partial{\textbf{f}(\textbf{v}_0)}}{\partial{\textbf{v}}}}
\newcommand{\pdgu}{\frac{\partial{\textbf{g}}}{\partial{\bV}}}

%PDE's mixed

\newcommand{\pdvoxy}{\frac{\partial^2{\textbf{v}_0}}{\partial{x}\partial{y}}}
\newcommand{\pdvoxth}{\frac{\partial^2{\textbf{v}_0}}{\partial{x}\partial{\theta}}}
\newcommand{\pdvoyx}{\frac{\partial^2{\textbf{v}_0}}{\partial{y}\partial{x}}}
\newcommand{\pdvoyth}{\frac{\partial^2{\textbf{v}_0}}{\partial{y}\partial{\theta}}}
\newcommand{\pdvothx}{\frac{\partial^2{\textbf{v}_0}}{\partial{\theta}\partial{x}}}
\newcommand{\pdvothy}{\frac{\partial^2{\textbf{v}_0}}{\partial{\theta}\partial{y}}}
